# Supplementary material for: A Gated Fusion Network for Dynamic Saliency Prediction
Source: arXiv:2102.07682 source file (2021-02-15)
Supplement: Supplementary file 1 [file supp.tex]

\title{Dynamic Fusion Networks \\ for  Predicting Saliency in Videos}
\author{Aysun Kocak, 
	Erkut Erdem
	and~Aykut Erdem}

\maketitle
\IEEEpeerreviewmaketitle
\begin{abstract}

\end {abstract}

\begin{keywords}

\end{keywords}

\section{Additional Experiments}
We will separate this part for supp. material. Just observe the results

\begin{table*}[ht]
	\centering
		\caption{Performance comparisons}
	\resizebox{\textwidth}{!}{\begin{tabular}{c|ccccc|ccccc}
		\hline
		\backslashbox{Class}{Method}&\multicolumn{5}{c}{Ours}&\multicolumn{5}{c}{ACLNet} \\
		&AUC-J & s-AUC & CC & NSS & SIM&AUC-J & s-AUC & CC & NSS & SIM\\ 
		\hline 
Diving-Side&0.952&0.856&0.840&4.641&0.646& 0.928&0.765&0.610&2.924&0.468\\
Golf-Swing-Front&0.896&0.764&0.461&2.478&0.399&0.900&0.739&0.483&2.195&0.401\\
Kicking-Front&0.907&0.767&0.569&2.638&0.474&0.878&0.627&0.450&1.874& 0.411\\
Lifting&0.939&0.756&0.850&4.649&0.667 & 0.926&0.749&0.711&3.196&0.531 \\
Riding-Horse&0.874&0.82&0.702&2.514&0.584&0.802& 0.403& 0.247&0.756&0.340\\
Run-Side&0.901&0.755&0.697&2.829&0.562&0.888&0.646& 0.566& 2.013&0.494\\
SkateBoarding-Front&0.933&0.770&0.622&3.054&0.522&0.810&0.540&0.392&1.629&0.366\\
Swing-Bench&0.906&0.734&0.688&2.799&0.561&0.891&0.673&0.599&2.207& 0.501\\
Swing-SideAngle&0.944&0.822&0.883&4.889&0.679&0.922&0.729 & 0.611& 2.728&0.445\\
Walk-Front&0.898&0.775&0.685&2.863&0.545 &0.849&0.550&0.419&1.505&0.400\\
		\hline
	\end{tabular}}
	\label{tab:results}
\end{table*}

\begin{table*}[ht]
	\centering
		\caption{Performance comparisons}
	\resizebox{\textwidth}{!}{\begin{tabular}{c|ccccc|ccccc}
		\hline
		\backslashbox{Class}{Method}&\multicolumn{5}{c}{Ours}&\multicolumn{5}{c}{ACLNet} \\
		&AUC-J & s-AUC & CC & NSS & SIM&AUC-J & s-AUC & CC & NSS & SIM\\ 
		\hline 
		
advert\_bbc4\_bees\_1024x576&0.731&0.541&0.488&2.0738&0.405&0.861&0.467&0.433&1.745&0.352 \\
advert\_bbc4\_library\_1024x576&0.710&0.430&0.323&1.268&0.323&0.827&0.476&0.375&1.493&0.346 \\
advert\_iphone\_1272x720&0.853&0.637&0.471&2.311&0.377 &0.940&0.691&0.525&2.491&0.353\\
BBC\_life\_in\_cold\_blood\_1278x710&0.848&0.643&0.498&2.0601&0.422&0.908&0.602&0.543&2.157&0.433\\
BBC\_wildlife\_serpent\_1280x704&0.821&0.570&0.469&1.776&0.397 &0.873&0.469&0.398&1.430&0.359\\
DIY\_SOS\_1280x712&0.742&0.619&0.385&1.639&0.349&0.892&0.572&0.457&1.888&0.398\\
harry\_potter\_6\_trailer\_1280x544&0.894&0.694&0.651&2.740&0.505&0.947&0.712&0.650&2.599&0.446\\
music\_gummybear\_880x720&0.802&0.579&0.436&1.737&0.376 &0.919&0.572&0.470&1.863&0.376\\
music\_trailer\_nine\_inch\_nails\_1280x720&0.856&0.647&0.534&2.395&0.414&0.858&0.488&0.441&1.703&0.340 \\
nightlife\_in\_mozambique\_1280x580&0.871&0.619&0.565&1.935&0.464&0.926&0.606&0.632&2.131&0.477 \\
one\_show\_1280x712&0.964&0.908&0.863&5.969&0.618&0.983&0.928&0.852&5.657&0.565 \\
pingpong\_angle\_shot\_960x720&0.895&0.735&0.598&2.227&0.482&0.916&0.692&0.527&1.877&0.461 \\
pingpong\_no\_bodies\_960x720&0.706&0.467&0.405&1.304&0.379&0.849&0.481&0.473&1.457&0.428 \\
sport\_scramblers\_1280x720&0.861&0.721&0.648&3.176&0.500&0.917&0.654&0.579&2.552&0.419\\
sport\_wimbledon\_federer\_final\_1280x704&0.828&0.650&0.492&1.946&0.412&0.870&0.525&0.388&1.528&0.339 \\
university\_forum\_construction\_ionic\_1280x720&0.741&0.575&0.341&1.308&0.326&0.892&0.604&0.502&1.821&0.393 \\
		\hline
	\end{tabular}}
	\label{tab:results}
\end{table*}

\bibliographystyle{IEEEtran}
\bibliography{06_Bibliography_Clean}
